# Supplementary material for: Fair and Efficient Multi-Resource Allocation for Cloud Computing
Source: arXiv:2210.05237 source file (2022-10-11)
Supplement: Supplementary file 1 [file appendix.tex]

% !TEX root = DRF-arXiv.tex

\section{Proofs}

\subsection{Proof of Lemma \ref{lem:n-2-DRF}}

\DRF*

\subsection{Proof of Theorem \ref{thm:n-2-F1}}

\FONE*

\subsection{Proof of Theorem \ref{thm:n-2-F2}}
\label{sec:proof-F2}

% We first present Algorithm \ref{alg:F2-step}, which computes the increasing steps $(\delta^*_1,\delta^*_2)$ (CalcStep $()$ in line 10 of Algorithm \ref{alg:F2}).

% \begin{algorithm}[]
%     \DontPrintSemicolon
%     % \KwInput{$\mathbf{A},\mathbf{d}_i,C,G_1,G_2,P_1,P_2,R_1,R_2$}
%     % \KwOutput{$(\delta^*_1,\delta^*_2)$}
    
%       \ForEach{$k = 1,2$}
%       {
%         $\delta_k \leftarrow \min\limits_{i \in N \setminus P_k} A_{i,3-k}-\min\limits_{i \in P_k} A_{i,3-k}$ \tcp*{increasing step when 2nd smallest fraction of resource $r_{3-k}$ is reached}
%         $D_k \leftarrow \sum_{i \in P_k} \frac{1}{d_{i,3-k}}$ \\
%         $\overline{\delta_k} \leftarrow \frac{c_{3-k}}{|P_k|+ D_k\frac{R_{3-k}}{R_k}}$
%         \tcp*{increasing step when resource $r_{3-k}$ is used up}
%         $\delta_k^* \leftarrow \min\{\delta_k,\overline{\delta_k}\}$
%       }
%       \If{$\frac{\delta_1^* D_1}{\delta_2^* D_2} \le \frac{R_1}{R_2}$}
%       {
%         $\delta_2^* \leftarrow \delta_1^* \cdot \frac{ D_1}{D_2} \cdot \frac{R_2}{R_1}$ \tcp*{decrease $\delta_2^*$ according to $\delta_1^*$}
%       }
%       \Else
%       {
%         $\delta_1^* \leftarrow \delta_2^* \cdot \frac{D_2}{D_1} \cdot \frac{R_1}{R_2}$ \tcp*{decrease $\delta_1^*$ according to $\delta_2^*$}
%       }
%       \Return $(\delta^*_1,\delta^*_2)$
%     \caption{CalcStep $()$}
%     \label{alg:F2-step}
%     \end{algorithm}

\FTWO*

% \begin{lemma}
% \label{lem:F2-not-SP}
% $\FTwo$ does not satisfy SP.
% \end{lemma}

% \begin{proof}
% Consider an instance with two agents and their demand vectors are $\mathbf{d}_1=(1,\frac{1}{2})$ and $\mathbf{d}_2=(\frac{1}{4},1)$.
% According to $\FTwo$, agent 1 gets $(\frac{1}{2},\frac{1}{4})$ and agent 2 gets $(\frac{1}{8},\frac{1}{2})$ in step 1.
% Then the remaining resources is $(\frac{3}{8},\frac{1}{4})$ and the increasing speed ratio is $\frac{3}{2}$.
% In step 2, agent 1 gets $(\frac{3}{14},\frac{3}{28})$ and agent 2 gets $(\frac{1}{28},\frac{1}{7})$, and resource~2 is used up.
% Overall agent 2 gets $(\frac{9}{56},\frac{9}{14})$.

% If agent 2 reports another demand vector $\mathbf{d}'_2=(\frac{1}{2},1)$, then two agents will get the same dominant share $\frac{2}{3}$ under $\FTwo$.
% In particular, agent 2 will get $(\frac{1}{3},\frac{2}{3})$, which is strictly larger than $(\frac{9}{56},\frac{9}{14})$.
% Therefore, $\FTwo$ is not SP.
% \end{proof}

\subsection{Proof of Theorem \ref{thm:n-2-F2s}}
\label{sec:proof-F2s}

\FTWOS*

\subsection{Proof of Theorem \ref{thm:F-family}}

\FG*

% \begin{lemma}
% \label{lemma:F-family-property}
% All mechanisms from $\mathcal{F}$ satisfy SI, EF, PO, and SP.
% \end{lemma}

\subsection{Proof of Theorem \ref{thm:n-m-F1}}

\GFONE*

\subsection{Proof of Theorem \ref{thm:n-2-SP}}

\TWORSP*

\subsection{Proof of Theorem \ref{thm:lower-bound}}

\LBOUND*

\section{Experimental evaluation of generalized $\FOne$ and DRF for $m \ge 3$}
\label{sec:exp-m=3}
